# Supplementary material for: Diffusion Models for Constrained Domains
Source: arXiv:2304.05364 source file (2024-03-07)
Supplement: Supplementary file 1 [file technical_appendix.tex]

\section{Hessian Manifolds}

For actually computing the $g^{-1/2}$ we compute $U, S, V = svd(g(x))$ and then let $g^{-1/2} = U Diag(S^{-1/2}) V$ which requires $O(n^3)$ computations.
